# Supplementary material for: Unidentified Gamma-ray Sources as Targets for Indirect Dark Matter Detection with the Fermi-Large Area Telescope
Source: arXiv:1906.11896 ancillary file (2019-06-27)
Supplement: Supplementary file 1 [file Supplementary_table_of_unIDs.pdf]

| 3FGL Name | 2FHL Name | 3FHL Name | Rejection |
|---|---|---|---|
| 3FGL J0000.2-3738 | - | - | MW, ML |
| 3FGL J0001.6+3535 | - | - | ML |
| 3FGL J0002.0-6722 | - | - | ML |
| 3FGL J0002.6+6218 | - | - | A |
| 3FGL J0003.4+3100 | - | - | - |
| 3FGL J0004.2+0843 | - | - | MW, ML |
| 3FGL J0006.2+0135 | - | - | MW, ML |
| 3FGL J0006.6+4618 | - | - | ML |
| 3FGL J0007.4+1742 | - | - | ML |
| 3FGL J0007.9+4006 | - | - | ML |
| 3FGL J0008.3+1456 | - | - | MW |
| 3FGL J0010.5-1425 | - | - | ML |
| 3FGL J0014.3-0455 | - | - | ML |
| 3FGL J0016.5+1713 | - | - | ML |
| 3FGL J0017.1+1445 | - | - | MW, ML |
| 3FGL J0020.9+0323 | - | - | MW, ML |
| 3FGL J0022.7+4651 | - | - | ML |
| 3FGL J0026.2-4812 | - | - | ML |
| 3FGL J0031.2-2320 | - | - | ML |
| 3FGL J0031.6+0938 | - | - | MW, ML |
| 3FGL J0032.3-5522 | - | - | V |
| 3FGL J0032.5+3912 | - | - | MW, ML |
| 3FGL J0048.1-6343 | - | - | MW |
| 3FGL J0049.0+4224 | - | 3FHL J0049.0+4224 | A, ML |
| 3FGL J0102.1+4458 | - | - | ML |
| 3FGL J0102.1+0943 | - | - | A, ML |
| 3FGL J0112.9-7506 | - | - | ML |
| 3FGL J0114.8+1917 | - | - | ML |
| 3FGL J0121.8-3917 | - | 3FHL J0121.9-3917 | A, MW |
| 3FGL J0127.6+4851 | - | - | ML |
| 3FGL J0132.1-5340 | - | - | MW, ML |
| 3FGL J0133.2-4737 | - | - | ML |
| 3FGL J0138.5-4612 | - | - | MW, ML |
| 3FGL J0149.6+4846 | - | - | MW, ML |
| 3FGL J0154.1+4642 | - | - | ML |
| 3FGL J0156.5-2423 | - | 3FHL J0156.2-2419 | A, ML |
| 3FGL J0158.6+0102 | - | - | A, ML |
| 3FGL J0200.3-4108 | - | - | A, ML |
| 3FGL J0203.6+1148 | - | - | MW, ML |
| 3FGL J0211.0+1922 | - | - | ML |
| 3FGL J0216.0+0300 | - | - | MW, ML |
| 3FGL J0216.4+0507 | - | - | ML |
| 3FGL J0221.2+2518 | - | 3FHL J0221.4+2512 | A, ML |
| 3FGL J0223.6+3927 | - | - | ML |
| 3FGL J0224.1-1846 | - | 3FHL J0223.9-1850 | MW, ML |
| 3FGL J0224.4+1615 | - | - | ML |
| 3FGL J0226.7-4747 | - | - | ML |
| 3FGL J0228.5+8213 | - | - | ML |
| 3FGL J0231.0+1302 | - | - | ML |
| 3FGL J0232.6+0646 | - | 3FHL J0233.5+0657 | ML |
| 3FGL J0234.2-0629 | - | - | A, ML |
| 3FGL J0239.0+2555 | - | - | A, ML |
| 3FGL J0239.4+1326 | - | - | ML |
| 3FGL J0240.0-0253 | - | - | ML |
| 3FGL J0242.1-0534 | - | - | ML |

Table XXX – Continued.

| 3FGL Name | 2FHL Name | 3FHL Name | Rejection |
|---|---|---|---|
| 3FGL J0244.4+4745 | - | - | - |
| 3FGL J0251.1-1829 | - | 3FHL J0251.2-1830 | MW, ML |
| 3FGL J0258.2+3555 | - | - | ML |
| 3FGL J0258.9+0552 | - | 3FHL J0258.9+0554 | MW, ML |
| 3FGL J0307.3+4916 | - | - | A |
| 3FGL J0308.4-2852 | - | - | ML |
| 3FGL J0312.1-0921 | - | - | A |
| 3FGL J0312.7-2222 | - | - | A, ML |
| 3FGL J0312.7+2011 | - | 3FHL J0312.7+2013 | ML |
| 3FGL J0318.1+0252 | - | - | MW |
| 3FGL J0322.5-3721 | - | - | ML |
| 3FGL J0323.7-6038 | - | - | ML |
| 3FGL J0324.5-1315 | - | - | ML |
| 3FGL J0330.6+0437 | - | - | MW, ML |
| 3FGL J0333.6+0233 | - | - | MW, ML |
| 3FGL J0336.1+7500 | - | - | - |
| 3FGL J0340.4-2423 | - | - | A, ML |
| 3FGL J0342.8+1321 | - | - | MW, ML |
| 3FGL J0345.3+3236 | - | - | MW |
| 3FGL J0351.0-2816 | - | 3FHL J0350.8-2814 | A, ML |
| 3FGL J0351.4-3248 | - | - | ML |
| 3FGL J0359.5+5413 | - | - | A |
| 3FGL J0359.7+7649 | - | - | MW, ML |
| 3FGL J0401.0-5359 | - | - | MW, ML |
| 3FGL J0402.7+2616 | - | - | ML |
| 3FGL J0412.0+0229 | - | - | MW, ML |
| 3FGL J0414.9-0840 | - | - | A, ML |
| 3FGL J0415.7-4351 | - | - | A, ML |
| 3FGL J0418.2+3412 | - | - | MW, ML |
| 3FGL J0419.1+6636 | - | - | MW |
| 3FGL J0420.4+1448 | - | - | ML |
| 3FGL J0420.4-6013 | - | - | A, ML |
| 3FGL J0420.6-3742 | - | - | ML |
| 3FGL J0421.6+1950 | - | - | MW, ML |
| 3FGL J0427.9-6704 | - | 3FHL J0427.5-6705 | MW, ML |
| 3FGL J0430.1-3103 | - | - | MW, ML |
| 3FGL J0432.5+0539 | - | - | MW, ML |
| 3FGL J0437.7-7330 | - | 3FHL J0438.0-7328 | A, ML |
| 3FGL J0447.1-2540 | - | - | MW, ML |
| 3FGL J0451.6+7231 | - | - | MW, ML |
| 3FGL J0456.2-6924 | - | - | ML |
| 3FGL J0502.6+1759 | - | - | ML |
| 3FGL J0506.3-0357 | - | - | A, V |
| 3FGL J0506.9+0321 | - | 3FHL J0506.9+0323 | MW, ML |
| 3FGL J0507.5-0906 | - | - | ML |
| 3FGL J0512.0-3737 | - | - | MW, ML |
| 3FGL J0514.6-4406 | - | - | ML |
| 3FGL J0516.6+1012 | - | - | MW, ML |
| 3FGL J0523.3-2528 | - | - | MW |

Table XXX – Continued.

| 3FGL Name | 2FHL Name | 3FHL Name | Rejection |
|---|---|---|---|
| 3FGL J0524.5-6937 | - | - | ML |
| 3FGL J0525.2-6614 | - | - | ML |
| 3FGL J0527.3+6647 | - | 3FHL J0527.5+6648 | ML |
| 3FGL J0533.2+5944 | - | - | ML |
| 3FGL J0533.8-3754 | - | - | MW, ML |
| 3FGL J0535.3-6559 | - | - | ML |
| 3FGL J0536.4-3347 | - | - | V |
| 3FGL J0537.0-7113 | - | - | ML |
| 3FGL J0537.0+0957 | - | - | V |
| 3FGL J0538.8-0341 | - | - | - |
| 3FGL J0539.2-0536 | - | - | - |
| 3FGL J0539.9-7553 | - | - | ML |
| 3FGL J0545.6+6019 | - | 3FHL J0545.8+6015 | MW |
| 3FGL J0550.3-4521 | - | - | ML |
| 3FGL J0557.7-0720 | - | - | MW, ML |
| 3FGL J0600.4-1934 | - | - | - |
| 3FGL J0605.0-0000 | - | - | MW, ML |
| 3FGL J0608.2-2306 | - | - | MW, ML |
| 3FGL J0608.6+5328 | - | - | ML |
| 3FGL J0609.6-2851 | - | - | ML |
| 3FGL J0609.7-1841 | - | - | MW, ML |
| 3FGL J0623.1-4143 | - | - | MW, ML |
| 3FGL J0636.7+7115 | - | - | ML |
| 3FGL J0638.4+5704 | - | - | ML |
| 3FGL J0639.9+3250 | - | - | ML |
| 3FGL J0644.6+6035 | - | - | A, ML |
| 3FGL J0650.9+6524 | - | - | ML |
| 3FGL J0657.6-4701 | - | - | MW, ML |
| 3FGL J0658.8+2318 | - | - | MW, ML |
| 3FGL J0700.6+3557 | - | - | MW |
| 3FGL J0704.3-4828 | - | - | A, ML |
| 3FGL J0707.5-3111 | - | - | ML |
| 3FGL J0708.7+1747 | - | - | MW, ML |
| 3FGL J0712.2-3806 | - | - | ML |
| 3FGL J0714.7-3924 | - | - | MW, ML |
| 3FGL J0716.0-4525 | - | - | MW, ML |
| 3FGL J0718.9-5004 | - | - | ML |
| 3FGL J0721.5-0221 | - | - | A |
| 3FGL J0725.4-5007 | - | 3FHL J0725.6-5008 | MW, ML |
| 3FGL J0733.3+5904 | - | - | V |
| 3FGL J0737.8-8245 | - | - | ML |
| 3FGL J0739.8+1312 | - | - | ML |
| 3FGL J0740.6-5230 | - | - | MW, ML |
| 3FGL J0744.3+1715 | - | - | V |
| 3FGL J0746.4-0225 | - | - | ML |
| 3FGL J0747.5-4927 | - | 3FHL J0747.7-4927 | A, ML |
| 3FGL J0748.7-5116 | - | - | MW, ML |
| 3FGL J0749.0+4459 | - | - | V |
| 3FGL J0749.5+1320 | - | - | MW, ML |
| 3FGL J0757.5-0536 | - | - | MW |
| 3FGL J0802.3-5610 | - | - | V, ML |
| 3FGL J0802.3-0941 | - | - | ML |
| 3FGL J0810.5-5214 | - | - | MW, ML |
| 3FGL J0813.5-0356 | - | 3FHL J0813.7-0353 | MW, ML |
| 3FGL J0818.0+3237 | - | - | MW, ML |

Table XXX – Continued.

| 3FGL Name | 2FHL Name | 3FHL Name | Rejection |
|---|---|---|---|
| 3FGL J0823.6-4838 | - | - | V |
| 3FGL J0826.3-6400 | - | - | A, ML |
| 3FGL J0830.8+2629 | - | - | ML |
| 3FGL J0834.6+6101 | - | - | MW, ML |
| 3FGL J0843.4+6713 | - | - | A, ML |
| 3FGL J0846.8-2638 | - | - | MW, ML |
| 3FGL J0847.2-6936 | - | - | MW, ML |
| 3FGL J0848.5+7018 | - | - | MW, ML |
| 3FGL J0855.4+7142 | - | - | A, V |
| 3FGL J0856.4+6429 | - | - | MW, ML |
| 3FGL J0900.0+6754 | - | - | A, ML |
| 3FGL J0901.0-6725 | - | - | ML |
| 3FGL J0905.8-2127 | - | - | - |
| 3FGL J0919.4+6604 | - | - | MW, ML |
| 3FGL J0919.5-2200 | - | - | ML |
| 3FGL J0921.6+2339 | - | - | ML |
| 3FGL J0930.7+5133 | - | - | MW, ML |
| 3FGL J0931.8+6739 | - | - | MW, ML |
| 3FGL J0935.1-1736 | - | - | MW, ML |
| 3FGL J0935.2+0903 | - | - | MW, ML |
| 3FGL J0936.3-2114 | - | - | MW, ML |
| 3FGL J0937.9-1435 | - | 3FHL J0937.8-1434 | A, ML |
| 3FGL J0940.6-7609 | - | - | ML |
| 3FGL J0941.0+6151 | - | - | MW, ML |
| 3FGL J0946.2+5209 | - | - | ML |
| 3FGL J0948.1-3641 | - | - | ML |
| 3FGL J0950.4+7550 | - | - | MW, ML |
| 3FGL J0952.8+0711 | - | - | A, ML |
| 3FGL J0953.7-1510 | - | - | - |
| 3FGL J0954.8-3948 | - | - | A, ML |
| 3FGL J1002.0-2837 | - | - | ML |
| 3FGL J1013.4-4008 | - | - | A, ML |
| 3FGL J1016.6-4244 | - | 3FHL J1016.2-4245 | A, ML |
| 3FGL J1016.9-2653 | - | - | ML |
| 3FGL J1027.8+8253 | - | - | ML |
| 3FGL J1028.3-7419 | - | - | ML |
| 3FGL J1033.0-5945 | - | - | A |
| 3FGL J1035.7-6720 | - | - | A |
| 3FGL J1036.4-4348 | - | - | ML |
| 3FGL J1038.0-2425 | - | - | ML |
| 3FGL J1039.5+7324 | - | - | ML |
| 3FGL J1045.5-2335 | - | - | MW, ML |
| 3FGL J1047.8-3737 | - | 3FHL J1047.9-3738 | MW, ML |
| 3FGL J1049.7+1548 | - | - | A, ML |
| 3FGL J1050.4+0435 | - | - | V |
| 3FGL J1051.0+5332 | - | - | ML |
| 3FGL J1052.0+0816 | - | - | MW, ML |
| 3FGL J1054.2-3123 | - | - | ML |
| 3FGL J1056.7-5853 | - | - | A |
| 3FGL J1057.6-4051 | - | 3FHL J1057.6-4051 | MW, ML |
| 3FGL J1059.3+0224 | - | - | MW, ML |
| 3FGL J1100.2-2044 | - | - | A, ML |
| 3FGL J1103.3+5239 | - | - | A, ML |
| 3FGL J1104.9-6036 | - | - | A |
| 3FGL J1105.7+4427 | - | - | A, ML |

Table XXX – Continued.

| 3FGL Name | 2FHL Name | 3FHL Name | Rejection |
|---|---|---|---|
| 3FGL J1106.6-1744 | - | - | - |
| 3FGL J1112.1+0500 | - | - | ML |
| 3FGL J1112.1+1034 | - | - | A, ML |
| 3FGL J1113.1-4515 | - | - | MW, ML |
| 3FGL J1115.0-0701 | - | 3FHL J1115.2-0705 | V |
| 3FGL J1116.7-4854 | - | - | ML |
| 3FGL J1117.7+0217 | - | - | MW, ML |
| 3FGL J1119.8-2647 | - | - | MW, ML |
| 3FGL J1119.9-2204 | - | - | MW |
| 3FGL J1120.6+0713 | - | - | MW |
| 3FGL J1123.3-2529 | - | - | A, ML |
| 3FGL J1123.6-4558 | - | - | ML |
| 3FGL J1125.1-5803 | - | - | A |
| 3FGL J1126.8-5001 | - | - | MW |
| 3FGL J1128.7-6232 | - | - | A |
| 3FGL J1129.0+3758 | - | - | A, ML |
| 3FGL J1130.7-7800 | - | - | MW, ML |
| 3FGL J1132.0-4736 | - | - | A, ML |
| 3FGL J1146.1-0640 | - | 3FHL J1145.9-0637 | MW, ML |
| 3FGL J1149.1+2815 | - | - | MW, ML |
| 3FGL J1150.7-4816 | - | - | MW, ML |
| 3FGL J1151.5+0957 | - | - | ML |
| 3FGL J1155.3-1112 | - | - | MW, ML |
| 3FGL J1200.4+0202 | - | 3FHL J1200.3+0201 | MW, ML |
| 3FGL J1200.9-1432 | - | - | MW, ML |
| 3FGL J1203.9-1745 | - | - | MW, ML |
| 3FGL J1205.9+3315 | - | - | MW, ML |
| 3FGL J1209.9+7607 | - | - | ML |
| 3FGL J1210.1-2742 | - | - | V |
| 3FGL J1211.8+6413 | - | - | MW, ML |
| 3FGL J1213.9-4412 | - | - | ML |
| 3FGL J1214.4-2315 | - | - | MW, ML |
| 3FGL J1215.9-1926 | - | - | ML |
| 3FGL J1216.6-0557 | - | - | ML |
| 3FGL J1220.0-2502 | - | 3FHL J1220.1-2459 | MW, ML |
| 3FGL J1220.1-3715 | - | 3FHL J1220.4-3714 | MW, ML |
| 3FGL J1220.3+6055 | - | 3FHL J1220.4+6053 | MW, ML |
| 3FGL J1221.5-0632 | - | - | A, ML |
| 3FGL J1222.7+7952 | - | - | A, ML |
| 3FGL J1223.2+1215 | - | - | MW, ML |
| 3FGL J1223.3+0818 | - | - | MW, ML |
| 3FGL J1225.4-3448 | - | - | MW, ML |
| 3FGL J1225.9+2953 | - | - | - |
| 3FGL J1228.4-0317 | - | - | MW, ML |
| 3FGL J1231.6-5113 | - | - | MW |
| 3FGL J1231.6+4825 | - | - | MW, ML |
| 3FGL J1232.3+1701 | - | - | MW, ML |
| 3FGL J1232.5-3720 | - | - | MW, ML |
| 3FGL J1232.8+1332 | - | - | MW, ML |
| 3FGL J1234.7-0437 | - | 3FHL J1234.8-0435 | MW, ML |
| 3FGL J1239.1-1158 | - | - | ML |
| 3FGL J1249.1-2808 | - | 3FHL J1249.2-2809 | ML |
| 3FGL J1249.5-0546 | - | - | MW, ML |
| 3FGL J1250.2-0233 | - | - | MW, ML |
| 3FGL J1251.0-4943 | - | - | ML |

Table XXX – Continued.

| 3FGL Name | 2FHL Name | 3FHL Name | Rejection |
|---|---|---|---|
| 3FGL J1257.0-6338 | - | - | V |
| 3FGL J1258.4+2123 | - | - | ML |
| 3FGL J1259.3-8151 | - | - | MW, ML |
| 3FGL J1259.5-3231 | - | - | ML |
| 3FGL J1301.5+3333 | - | - | A, ML |
| 3FGL J1304.6+1200 | - | - | ML |
| 3FGL J1306.8-4031 | - | - | A, ML |
| 3FGL J1309.0+0347 | - | - | MW, ML |
| 3FGL J1312.3+8513 | - | - | MW, ML |
| 3FGL J1315.7-0732 | - | - | ML |
| 3FGL J1316.2-6446 | - | - | V |
| 3FGL J1323.2-3901 | - | - | MW, ML |
| 3FGL J1325.2-5411 | - | - | A |
| 3FGL J1326.2-4651 | - | - | MW, ML |
| 3FGL J1329.1-0536 | - | - | ML |
| 3FGL J1330.4+5641 | - | - | A, ML |
| 3FGL J1333.8-4417 | - | - | ML |
| 3FGL J1334.3-4152 | - | - | A, ML |
| 3FGL J1335.2-4056 | - | - | ML |
| 3FGL J1345.1+1949 | - | - | ML |
| 3FGL J1346.2-2608 | - | - | MW, ML |
| 3FGL J1350.4-6224 | - | - | A |
| 3FGL J1351.1-2743 | - | - | MW, ML |
| 3FGL J1351.8-1524 | - | - | ML |
| 3FGL J1400.2-2413 | - | - | MW |
| 3FGL J1402.7-3240 | - | - | ML |
| 3FGL J1403.1+1304 | - | - | A, MW |
| 3FGL J1408.0-2924 | - | - | MW |
| 3FGL J1409.2-3743 | - | - | ML |
| 3FGL J1410.9+7406 | - | 3FHL J1410.8+7406 | ML |
| 3FGL J1411.1+3717 | - | - | A, ML |
| 3FGL J1411.4-0724 | - | - | A, ML |
| 3FGL J1417.5-4402 | - | - | ML |
| 3FGL J1417.7-5026 | - | - | MW, ML |
| 3FGL J1420.9-4615 | - | - | MW, ML |
| 3FGL J1421.0-2431 | - | - | MW |
| 3FGL J1421.8-7920 | - | - | ML |
| 3FGL J1424.3-1753 | - | - | ML |
| 3FGL J1427.2+1610 | - | - | ML |
| 3FGL J1430.8-4434 | - | - | MW, ML |
| 3FGL J1438.6-4209 | - | - | MW, ML |
| 3FGL J1458.7-2120 | - | - | V |
| 3FGL J1502.2+5553 | - | - | V |
| 3FGL J1506.4-0340 | - | - | MW, ML |
| 3FGL J1512.3+6622 | - | - | MW, ML |
| 3FGL J1512.8-5639 | - | - | V |
| 3FGL J1513.3-3719 | - | 3FHL J1513.4-3721 | MW, ML |
| 3FGL J1517.0+2637 | - | 3FHL J1517.0+2638 | MW, ML |
| 3FGL J1517.6-4442 | - | - | ML |
| 3FGL J1517.6-4442 | - | - | ML |
| 3FGL J1525.8-0834 | - | - | MW, ML |
| 3FGL J1527.0-3804 | - | - | MW, ML |
| 3FGL J1528.1-2904 | - | - | MW, ML |
| 3FGL J1528.3-5836 | - | - | A |
| 3FGL J1528.7-2247 | - | - | ML |

Table XXX – Continued.

| 3FGL Name | 2FHL Name | 3FHL Name | Rejection |
|---|---|---|---|
| 3FGL J1529.5+6733 | - | - | MW, ML |
| 3FGL J1532.0-2618 | - | - | MW, ML |
| 3FGL J1539.2-3324 | - | - | MW |
| 3FGL J1541.6+1414 | - | 3FHL J1541.7+1413 | MW, ML |
| 3FGL J1543.5-0244 | - | - | - |
| 3FGL J1544.1-2555 | - | - | MW |
| 3FGL J1544.6-1125 | - | - | A |
| 3FGL J1548.4+1455 | - | - | A, ML |
| 3FGL J1549.9-3044 | - | - | MW, ML |
| 3FGL J1550.4+6027 | - | 3FHL J1550.7+6027 | MW, ML |
| 3FGL J1553.1+5437 | - | - | A, ML |
| 3FGL J1601.9+2306 | - | - | MW |
| 3FGL J1602.8-1924 | - | 3FHL J1602.8-1928 | ML |
| 3FGL J1611.9+1404 | - | - | A, ML |
| 3FGL J1616.8+5846 | - | - | ML |
| 3FGL J1618.8+5520 | - | - | ML |
| 3FGL J1619.1+7538 | - | - | MW, ML |
| 3FGL J1622.9-5004 | - | - | A |
| 3FGL J1624.2-4041 | - | - | A |
| 3FGL J1625.1-0021 | - | - | A, MW |
| 3FGL J1625.2-2845 | - | - | MW, ML |
| 3FGL J1625.6-2058 | - | - | MW, ML |
| 3FGL J1627.8+3217 | - | - | A |
| 3FGL J1628.1-3344 | - | - | MW, ML |
| 3FGL J1628.1+0254 | - | - | MW, ML |
| 3FGL J1628.7-8056 | - | - | ML |
| 3FGL J1630.2-1052 | - | - | V, MW |
| 3FGL J1630.3-6126 | - | - | V |
| 3FGL J1632.8+3838 | - | - | MW, V |
| 3FGL J1635.3+4257 | - | - | ML |
| 3FGL J1640.6-4917 | - | - | V |
| 3FGL J1641.5-2856 | - | - | ML |
| 3FGL J1642.4+8045 | - | - | ML |
| 3FGL J1644.4+2632 | - | - | ML |
| 3FGL J1644.6-0911 | - | - | MW, ML |
| 3FGL J1645.7-2149 | - | - | A, V |
| 3FGL J1646.9-1332 | - | - | ML |
| 3FGL J1648.0+4230 | - | - | ML |
| 3FGL J1650.0+0356 | - | - | V |
| 3FGL J1650.3-4600 | - | - | A |
| 3FGL J1653.6-0158 | - | - | MW |
| 3FGL J1659.0-0142 | - | - | ML |
| 3FGL J1704.1+1234 | - | - | A, ML |
| 3FGL J1704.4-0528 | 2FHL J1704.7-0528 | 3FHL J1704.5-0527 | A, ML |
| 3FGL J1705.5+0948 | - | - | ML |
| 3FGL J1707.8+5626 | - | - | ML |
| 3FGL J1709.4-0917 | - | - | ML |
| 3FGL J1709.5-0335 | - | - | ML |
| 3FGL J1709.9+4624 | - | - | ML |
| 3FGL J1720.3-0428 | - | - | MW, ML |
| 3FGL J1720.7+0711 | - | - | MW |
| 3FGL J1722.7-0415 | - | - | MW |
| 3FGL J1725.0-0513 | - | - | MW, ML |
| 3FGL J1727.4+0634 | - | - | ML |
| 3FGL J1727.6-0654 | - | - | ML |

Table XXX – Continued.

| 3FGL Name | 2FHL Name | 3FHL Name | Rejection |
|---|---|---|---|
| 3FGL J1728.0-6446 | - | - | ML |
| 3FGL J1729.0+6049 | - | - | MW, ML |
| 3FGL J1729.9-0859 | - | - | MW |
| 3FGL J1730.6-0357 | - | - | A |
| 3FGL J1731.9+5428 | - | - | A, ML |
| 3FGL J1732.7+5914 | - | - | MW, ML |
| 3FGL J1733.8-6056 | - | - | MW, ML |
| 3FGL J1740.8-6755 | - | - | MW, ML |
| 3FGL J1741.4+0938 | - | - | ML |
| 3FGL J1742.4-7237 | - | - | ML |
| 3FGL J1744.1-7619 | - | - | A |
| 3FGL J1745.4+4721 | - | - | ML |
| 3FGL J1746.6+0433 | - | - | ML |
| 3FGL J1747.0-2828 | - | - | V |
| 3FGL J1747.3+0324 | - | - | ML |
| 3FGL J1748.0+2701 | - | - | MW, ML |
| 3FGL J1749.7-0305 | - | - | MW, ML |
| 3FGL J1757.7-6030 | - | - | V |
| 3FGL J1801.5-7825 | - | - | V |
| 3FGL J1803.3-6706 | - | 3FHL J1803.1-6709 | MW, ML |
| 3FGL J1804.1+2532 | - | - | MW, ML |
| 3FGL J1805.9+3407 | - | - | ML |
| 3FGL J1806.2+2744 | - | - | ML |
| 3FGL J1806.8+5346 | - | - | MW, ML |
| 3FGL J1809.0+3517 | - | - | MW, ML |
| 3FGL J1810.7+5335 | - | - | ML |
| 3FGL J1810.8-2412 | - | - | A |
| 3FGL J1813.6-6845 | - | - | ML |
| 3FGL J1813.6+2820 | - | - | MW, ML |
| 3FGL J1815.1+5919 | - | - | ML |
| 3FGL J1816.0-6407 | - | - | MW, ML |
| 3FGL J1817.7+2530 | - | - | ML |
| 3FGL J1818.5+1320 | - | - | ML |
| 3FGL J1819.5-1345 | - | - | V |
| 3FGL J1821.9+6636 | - | 3FHL J1821.4+6637 | MW, ML |
| 3FGL J1823.2-4722 | - | - | MW |
| 3FGL J1824.2-5427 | - | - | V |
| 3FGL J1827.3-1446 | - | - | A |
| 3FGL J1827.7+1141 | - | - | MW |
| 3FGL J1829.2+3229 | - | - | MW |
| 3FGL J1829.2+2731 | - | - | MW |
| 3FGL J1831.6-6503 | - | - | V, MW |
| 3FGL J1838.1+3827 | - | - | ML |
| 3FGL J1839.9+7646 | - | - | ML |
| 3FGL J1840.5+6116 | - | - | ML |
| 3FGL J1842.2+2742 | - | - | ML |
| 3FGL J1844.3-0344 | - | - | A |
| 3FGL J1845.5-2524 | - | - | MW, ML |
| 3FGL J1848.6+3232 | - | - | V |
| 3FGL J1857.0-7341 | - | - | ML |
| 3FGL J1857.9+7319 | - | 3FHL J1858.4+7318 | MW, ML |
| 3FGL J1857.9+5549 | - | - | ML |
| 3FGL J1858.0-5423 | - | - | ML |
| 3FGL J1911.1-5318 | - | - | ML |
| 3FGL J1912.7+4610 | - | - | ML |

Table XXX – Continued.

| 3FGL Name | 2FHL Name | 3FHL Name | Rejection |
|---|---|---|---|
| 3FGL J1917.1-3024 | - | - | ML |
| 3FGL J1921.6+1934 | - | - | A |
| 3FGL J1923.2-7452 | - | - | MW, ML |
| 3FGL J1924.8-1034 | - | - | ML |
| 3FGL J1925.8-7826 | - | - | ML |
| 3FGL J1934.2+6002 | - | - | MW, ML |
| 3FGL J1944.0-0535 | - | - | MW, ML |
| 3FGL J1945.3+7329 | - | - | ML |
| 3FGL J1946.4-5403 | - | - | A |
| 3FGL J1947.4-1121 | - | - | - |
| 3FGL J1947.9-0743 | - | - | MW, ML |
| 3FGL J1948.1-7059 | - | - | ML |
| 3FGL J1949.5-1454 | - | - | ML |
| 3FGL J1949.7-8109 | - | - | MW, ML |
| 3FGL J1951.3+6909 | - | - | MW, ML |
| 3FGL J1951.8-1102 | - | - | MW, ML |
| 3FGL J1953.4+7653 | - | - | MW, ML |
| 3FGL J1955.7-7019 | - | - | MW, ML |
| 3FGL J1957.9-0712 | - | - | MW, ML |
| 3FGL J1958.1-0243 | - | - | ML |
| 3FGL J1958.2-1413 | - | - | - |
| 3FGL J2005.7-8241 | - | - | MW, ML |
| 3FGL J2006.5-0939 | - | - | ML |
| 3FGL J2006.6+0150 | - | - | A, MW |
| 3FGL J2009.2-1458 | - | - | A, V, MW |
| 3FGL J2010.0-2120 | - | - | V, MW |
| 3FGL J2015.3-1431 | - | - | A, ML |
| 3FGL J2017.9+3627 | - | - | A |
| 3FGL J2022.2-7220 | - | - | MW, ML |
| 3FGL J2024.6+0309 | - | - | MW, ML |
| 3FGL J2024.8-2331 | - | - | MW, ML |
| 3FGL J2025.1-2858 | - | - | MW, ML |
| 3FGL J2026.3+1430 | - | - | MW, ML |
| 3FGL J2028.7+1012 | - | - | MW, ML |
| 3FGL J2029.5-4232 | - | - | - |
| 3FGL J2030.5-1439 | - | - | A, ML |
| 3FGL J2032.5+4032 | - | - | V |
| 3FGL J2034.6-4202 | - | - | ML |
| 3FGL J2038.8-3613 | - | - | A, ML |
| 3FGL J2039.6-5618 | - | - | A |
| 3FGL J2039.7+1237 | - | - | MW, ML |
| 3FGL J2042.3-5416 | - | - | ML |
| 3FGL J2043.6+0001 | - | - | MW, ML |
| 3FGL J2043.8-4801 | - | - | - |
| 3FGL J2044.0+1035 | - | - | MW, ML |
| 3FGL J2045.6-6838 | - | - | MW, ML |
| 3FGL J2046.7-4259 | - | - | ML |
| 3FGL J2047.9-3119 | - | - | MW, ML |
| 3FGL J2053.1+6027 | - | - | MW, ML |
| 3FGL J2053.4-4052 | - | - | ML |
| 3FGL J2054.3+6907 | - | - | MW |
| 3FGL J2054.8-4908 | - | - | MW |
| 3FGL J2055.6+1609 | - | - | MW, ML |
| 3FGL J2056.3-5925 | - | - | MW |
| 3FGL J2059.9+2029 | - | - | MW, ML |

Table XXX – Continued.

| 3FGL Name | 2FHL Name | 3FHL Name | Rejection |
|---|---|---|---|
| 3FGL J2100.6-7844 | - | - | ML |
| 3FGL J2103.7-1113 | - | - | V |
| 3FGL J2104.7+2113 | - | 3FHL J2104.5+2117 | ML |
| 3FGL J2107.1+2248 | - | - | ML |
| 3FGL J2109.4+1437 | - | - | V |
| 3FGL J2110.0+0442 | - | 3FHL J2109.7+0440 | MW, ML |
| 3FGL J2112.5-3044 | - | - | A, MW |
| 3FGL J2115.2+1215 | - | 3FHL J2115.2+1218 | A, ML |
| 3FGL J2116.9+1343 | - | - | MW, ML |
| 3FGL J2120.4-1256 | - | - | ML |
| 3FGL J2121.5-8253 | - | - | ML |
| 3FGL J2127.1-5615 | - | - | ML |
| 3FGL J2127.5-6001 | - | - | MW, ML |
| 3FGL J2130.4-4237 | - | - | V |
| 3FGL J2131.1-6625 | - | - | MW |
| 3FGL J2131.5+2605 | - | - | ML |
| 3FGL J2133.0-6433 | - | - | V, MW |
| 3FGL J2133.6+2821 | - | - | ML |
| 3FGL J2134.5-2131 | - | - | A, ML |
| 3FGL J2138.2-4939 | - | - | ML |
| 3FGL J2142.6-2029 | - | 3FHL J2142.5-2029 | MW, ML |
| 3FGL J2142.7+1957 | - | 3FHL J2142.7+1959 | MW, ML |
| 3FGL J2144.6-5640 | - | - | A, ML |
| 3FGL J2145.5+1007 | - | - | A, ML |
| 3FGL J2150.5-1754 | - | - | A, ML |
| 3FGL J2200.0-6930 | - | - | ML |
| 3FGL J2205.9-4704 | - | - | ML |
| 3FGL J2209.0+3652 | - | - | MW, ML |
| 3FGL J2209.8-0450 | - | - | A, MW |
| 3FGL J2210.1+5925 | - | - | A |
| 3FGL J2212.5+0703 | - | - | V, MW |
| 3FGL J2217.8+3207 | - | - | ML |
| 3FGL J2220.6-6833 | - | - | MW, ML |
| 3FGL J2223.3+0103 | - | - | A, ML |
| 3FGL J2224.4+0351 | - | - | MW, ML |
| 3FGL J2228.5-1636 | - | - | ML |
| 3FGL J2229.1+2255 | - | - | MW, ML |
| 3FGL J2237.5-8326 | - | - | A, MW |
| 3FGL J2244.6+2503 | - | - | A, ML |
| 3FGL J2247.2-0004 | - | - | MW, ML |
| 3FGL J2249.3-5943 | - | - | MW, ML |
| 3FGL J2250.3+1747 | - | - | V |
| 3FGL J2250.6+3308 | - | - | MW |
| 3FGL J2253.1-1237 | - | - | ML |
| 3FGL J2254.6+4253 | - | - | ML |
| 3FGL J2258.2-3645 | - | - | A, ML |
| 3FGL J2258.8+2437 | - | - | ML |
| 3FGL J2259.9-1553 | - | - | MW, ML |
| 3FGL J2300.0+4053 | - | - | MW, ML |
| 3FGL J2300.1-3547 | - | - | A, ML |
| 3FGL J2305.8+1658 | - | - | MW, ML |
| 3FGL J2310.1-0557 | - | - | A, V, MW |
| 3FGL J2313.1+3935 | - | - | ML |
| 3FGL J2318.6-3829 | - | - | MW, ML |
| 3FGL J2321.6-1619 | 2FHL J2321.6-1616 | 3FHL J2321.6-1618 | A, ML |

Table XXX – Continued.

| 3FGL Name | 2FHL Name | 3FHL Name | Rejection |
|---|---|---|---|
| 3FGL J2323.7+2523 | - | - | MW, ML |
| 3FGL J2327.2-4130 | - | - | ML |
| 3FGL J2331.9-1609 | - | - | ML |
| 3FGL J2333.0-5525 | - | - | MW |
| 3FGL J2334.4-7948 | - | - | ML |
| 3FGL J2335.6-2342 | - | - | ML |
| 3FGL J2337.2-8425 | - | - | A, ML |
| 3FGL J2337.5+4108 | - | - | MW, ML |
| 3FGL J2338.7+0251 | - | - | ML |
| 3FGL J2340.7+3847 | - | - | ML |
| 3FGL J2343.0-4748 | - | - | ML |
| 3FGL J2344.9-5647 | - | - | MW, ML |
| 3FGL J2351.9-7601 | 2FHL J2352.0-7558 | - | A |
| 3FGL J2354.0+2722 | - | - | MW, ML |
| 3FGL J2354.4-6612 | - | - | MW, ML |
| 3FGL J2354.8-5245 | - | - | V, MW |
| 3FGL J2358.5+3827 | - | - | MW, ML |
| 3FGL J2358.6-1809 | - | 3FHL J2358.4-1808 | A, ML |
| - | 2FHL J0213.9-6949 | 3FHL J0213.9-6950[1] | A |
| 3FGL J0310.4-5015[2] | 2FHL J0310.4-5019 | 3FHL J0310.6-5017 | A |
| 3FGL J0738.1+1741[3] | 2FHL J0738.6+1741 | - | A, MW, V |
| 3FGL J0746.6-4756 | 2FHL J0746.4-4757 | 3FHL J0746.6-4755[4] | A |
| 3FGL J0814.7+6428 | 2FHL J0814.8+6424 | 3FHL J0814.6+6429[5] | A |
| - | 2FHL J0845.7-5550 | 3FHL J0845.8-5551[6] | A |
| 3FGL J0912.9-2104[7] | 2FHL J0913.1-2058 | 3FHL J0912.9-2103 | A |
| - | 2FHL J1136.5-2721 | - | MW |
| - | 2FHL J1147.0-1437 | - | MW |
| 3FGL J1155.4-3417 | 2FHL J1155.5-3417 | 3FHL J1155.5-3418[8] | A |
| - | 2FHL J1421.4-4447 | - | A, MW, V |
| 3FGL J1427.8-3215[9] | 2FHL J1427.7-3215 | 3FHL J1427.7-3216 | A |
| - | 2FHL J1447.0-2658 | 3FHL J1447.0-2657[10] | A |
| - | 2FHL J1516.1+3702 | - | - |
| 3FGL J1545.0-6641[11] | 2FHL J1545.0-6641 | 3FHL J1544.9-6641 | A |
| 3FGL J1558.9-6432[12] | 2FHL J1559.2-6433 | 3FHL J1558.8-6432 | A |
| - | 2FHL J1630.0+7644 | - | - |
| - | 2FHL J1635.4-1414 | - | MW |
| - | 2FHL J1703.4-4145 | 3FHL J1703.4-4145[13] | A |
| - | 2FHL J1733.8-4733 | 3FHL J1733.8-4734[14] | A |
| 3FGL J1834.6-0659[15] | 2FHL J1834.6-0701 | 3FHL J1834.5-0846e | A |

[1] The 3FHL counterpart is not an unID
[2] The 3FGL and 3FHL counterparts are not unIDs
[3] The 3FGL counterpart is not an unID
[4] The 3FGL and 3FHL counterparts are not unIDs
[5] The 3FGL and 3FHL counterparts are not unIDs
[6] The 3FHL counterpart is not an unID
[7] The 3FGL and 3FHL counterparts are not unIDs
[8] The 3FHL counterpart is not an unID
[9] The 3FGL and 3FHL counterparts are not unIDs
[10] The 3FHL counterpart is not an unID
[11] The 3FGL and 3FHL counterparts are not unIDs
[12] The 3FGL and 3FHL counterparts are not unIDs
[13] The 3FHL counterpart is not an unID
[14] The 3FHL counterpart is not an unID
[15] The 3FGL and 3FHL counterparts are not unIDs

Table XXX – Continued.

| 3FGL Name | 2FHL Name | 3FHL Name | Rejection |
|---|---|---|---|
| - | 2FHL J1856.8+0256 | 3FHL J1857.7+0246e[16] | A |
| - | 2FHL J1912.9-4456 | - | MW |
| 3FGL J1628.2+7703[17] | 2FHL J2058.6-1832 | - | A, V |
| 3FGL J2108.6-8619[18] | 2FHL J2112.5-8617 | 3FHL J2111.0-8618 | A |
| - | 2FHL J2317.8+2838 | 3FHL J2317.8+2839 | MW |
| 3FGL J2351.9-7601[19] | 2FHL J2352.0-7558 | 3FHL J2351.5-7559 | A |
| - | - | 3FHL J0041.7-1608 | - |
| - | - | 3FHL J0055.8+4507 | - |
| - | - | 3FHL J0110.9+4346 | - |
| - | - | 3FHL J0115.4-2916 | - |
| - | - | 3FHL J0121.8+3808 | - |
| - | - | 3FHL J0158.8+3314 | V |
| - | - | 3FHL J0233.0+3742 | - |
| - | - | 3FHL J0243.3+1915 | V |
| - | - | 3FHL J0301.4-5618 | - |
| - | - | 3FHL J0302.6+3354 | - |
| 3FGL J0316.1-2611[20] | - | 3FHL J0316.5-2610 | A |
| - | - | 3FHL J0319.2-7045 | A |
| - | - | 3FHL J0327.6+2619 | MW |
| - | - | 3FHL J0343.5-6302 | - |
| - | - | 3FHL J0350.4-5143 | - |
| - | - | 3FHL J0359.4-0235 | - |
| - | - | 3FHL J0459.3+1921 | V |
| - | - | 3FHL J0500.6+1903 | V |
| - | - | 3FHL J0501.0+2425 | V |
| - | - | 3FHL J0540.2+0654 | V |
| - | - | 3FHL J0550.4-4356 | V, MW |
| - | - | 3FHL J0550.9+5657 | - |
| - | - | 3FHL J0620.9-5033 | - |
| - | - | 3FHL J0737.5+6534 | MW |
| - | - | 3FHL J0753.9+0452 | A |
| - | - | 3FHL J0838.5+4006 | - |
| - | - | 3FHL J0954.2-2520 | - |
| - | - | 3FHL J1212.2+2439 | V, MW |
| 3FGL J1248.0+5130[21] | - | 3FHL J1248.8+5128 | A |
| - | - | 3FHL J1403.4+4319 | - |
| - | - | 3FHL J1405.8-1854 | V, MW |
| 3FGL J1409.7-6132[22] | - | 3FHL J1409.1-6121e | A |
| - | - | 3FHL J1421.5-1654 | - |
| - | - | 3FHL J1427.9-6054 | - |
| 3FGL J1440.0-3955[23] | - | 3FHL J1439.9-3955 | A |
| - | - | 3FHL J1440.2-2343 | - |
| - | - | 3FHL J1441.3-1934 | - |
| - | - | 3FHL J1451.8-4145 | V |
| - | - | 3FHL J1503.3+1651 | - |
| - | - | 3FHL J1547.3-1530 | V |

[16] The 3FHL counterpart is not an unID
[17] The 3FGL counterpart is not an unID
[18] The 3FGL and 3FHL counterparts are not unIDs
[19] The 3FGL and 3FHL counterparts are not unIDs
[20] The 3FGL counterpart is not an unID
[21] The 3FGL counterpart is not an unID
[22] The 3FGL counterpart is not an unID
[23] The 3FGL counterpart is not an unID

Table XXX – Continued.

| 3FGL Name | 2FHL Name | 3FHL Name | Rejection |
|---|---|---|---|
| 3FGL J1553.3-2421[24] | - | 3FHL J1553.8-2425 | A |
| - | - | 3FHL J1648.1-1548 | MW |
| - | - | 3FHL J1650.9+0430 | - |
| - | - | 3FHL J1705.3+5434 | - |
| - | - | 3FHL J1716.1+2308 | - |
| - | - | 3FHL J1726.2-1710 | - |
| 3FGL J1745.1-3011[25] | - | 3FHL J1745.8-3028e | A |
| - | - | 3FHL J1753.9+2442 | MW |
| - | - | 3FHL J1808.7+2420 | A |
| - | - | 3FHL J1915.2-1323 | MW |
| - | - | 3FHL J1959.9-4606 | MW |
| - | - | 3FHL J2030.2-5037 | MW |
| - | - | 3FHL J2042.7+1520 | V |
| - | - | 3FHL J2105.9+7508 | MW |
| - | - | 3FHL J2110.2+0404 | MW |
| - | - | 3FHL J2142.3+3659 | A |
| - | - | 3FHL J2159.6-4619 | MW |
| - | - | 3FHL J2225.8-0803 | V, MW |
| - | - | 3FHL J2245.5-1734 | V, MW |

**Table XXX.** Rejection criteria for 3FGL, 2FHL and 3FHL unIDs. Last column indicates the rejection criteria: A=Association; V=Variable; ML=Machine learning; MW=Multiwavelength. Note that sources rejected by latitude or complex regions are not listed. Sources are only listed once, i.e., there is no duplicity between different catalogs. If more than one rejection criteria is cited, only the first is the used one.

[24] The 3FGL counterpart is not an unID

[25] The 3FGL counterpart is not an unID
